# Supplementary material for: Exploring Adversarial Robustness of Deep Metric Learning
Source: arXiv:2102.07265 source file (2021-02-14)
Supplement: Supplementary file 1 [file test_natural_attacks.tex]

\section{Experiment: Natural Robustness (Alternatives)}~\label{app:altattacks}
This section covers the robustness for naturally-trained \ac{DML} models for two other established attack methods, \ac{FGSM}~\citep{goodfellow14} and \ac{CW}~\citep{carlini17}.
Using the Algorithm~\ref{alg:attack} with these methods, it can be seen in Table~\ref{table:naturalattacks} that they also lower the performance for $\ell_{\infty}(\epsilon = 0.01)$.
Hyper-parameters for \ac{CW} are covered in Appendix~\ref{app:robustuni}, particularly iterations had to remain low to feasible runtime under the available resources.
Thereby, tuning parameters to a greater extend could yield a more powerful attack and thus lower robustness.

\begin{table*}
  \setlength{\tabcolsep}{4pt}
  \small
  \centering
  \begin{tabular}{
    l
    @{\hskip 2\tabcolsep}
    S[table-format=1.2, tight-spacing=true, table-text-alignment=left]
    *{3}{
    @{\hskip 4\tabcolsep}
    S[table-format=2.1, table-column-width=4em]
    S[table-format=2.1, table-column-width=4em]
    }}
    \toprule
     \parbox[t]{2mm}{\multirow{2}{*}{\rotatebox[origin=c]{90}{$\leftarrow$\small Loss}}} & \text{$\norm_{\infty}(\epsilon=0.01)$} & \multicolumn{2}{c}{\textbf{CUB200-2011}} & \multicolumn{2}{@{}c@{\hskip 4\tabcolsep}}{\textbf{CARS196}} & \multicolumn{2}{@{}c@{}}{\textbf{SOP}} \\
    \cmidrule(lr{\dimexpr 4\tabcolsep-0.5em}){3-4} \cmidrule(l{-0.5em}r{\dimexpr 4\tabcolsep-0.5em}){5-6} \cmidrule(l{-0.5em}r{0.5em}){7-8}
   & & {R@1} & {mAP@R} & {R@1} & {mAP@R} & {R@1} & {mAP@R}\\
    \midrule
    \parbox[t]{2mm}{\multirow{3}{*}{C}} & \textit{Benign} &           59.1 &                        21.0 &           74.0 &                        20.9 &           71.8 &                        44.7 \\
    \cmidrule(l{-0.5em}r{0.0em}){2-8}
     & \text{\ac{FGSM}} &           19.7 &                         7.2 &           14.6 &                         3.8 &           18.4 &                        10.8 \\
     & \text{\ac{CW}} &           15.1 &                         6.0 &            5.6 &                         2.3 &           23.1 &                        13.9 \\
    \midrule
    \parbox[t]{2mm}{\multirow{3}{*}{T}} & \textit{Benign} &           59.3 &                        21.7 &           74.0 &                        21.4 &           69.6 &                        42.1 \\
    \cmidrule(l{-0.5em}r{0.0em}){2-8}
     & \text{\ac{FGSM}} &           18.9 &                         7.7 &           15.5 &                         4.1 &           14.5 &                         8.5 \\
    & \text{\ac{CW}} &           22.9 &                        10.0 &           13.4 &                         3.6 &           10.0 &                         6.1 \\
    \bottomrule
  \end{tabular}
  \caption{\label{table:naturalattacks}
    Performance of naturally-trained \ac{DML} models against adversarial examples generated using Algorithm~\ref{alg:attack} with two alternative attack methods: \ac{FGSM} and \ac{CW}.
    Losses are denoted by C (contrastive) and T (triplet).
    Recall that, R@1 reflects a model's inference accuracy, while mAP@R reflects its ability to rank similar entities.
}
\end{table*}
