# Supplementary material for: Exploring Adversarial Robustness of Deep Metric Learning
Source: arXiv:2102.07265 source file (2021-02-14)
Supplement: Supplementary file 2 [file train_attacks.tex]

\section{Experiment: Universality of Robustness}\label{app:robustuni}

The robust \ac{DML} models trained using the proposed adversarial training algorithm (covered in Section~\ref{sec:advtrain}) approximate the solution to the $\argmax$ in $\rho((\datapoint_{i}, y_{i}),(\datapoint_{j},y_{j}),(\datapoint_{k},y_{k}))$ (\todo{defined in Equation~\ref{eq:rho}) using} \ac{PGD}~\citep{madry18}, and have demonstrated improved robustness towards attacks using on PGD (\todo{see Table~\ref{table:robust}}).
However, as a measure to test if the increased robustness also apply to attacks relying on other attack methods, such as \ac{FGSM} and \ac{CW}, \todo{we conduct a robustness evaluation using Algorithm~\ref{alg:attack}} with these two attack methods for $\norm_{\infty}(\epsilon = 0.01)$.
For \ac{FGSM}, we use $\alpha = \epsilon$, to maximize the perturbation, and thereby attack strength, under the given norm.
Despite \ac{CW} being originally designed for the $\norm_{2}$ norm, we sought out to adopt an implementation created by the author~\footnote{\ac{CW} for $\norm_{\infty}$, TensorFlow Implementation: \url{https://github.com/carlini/nn_robust_attacks/blob/master/li_attack.py}} for the $\norm_{\infty}$ norm.
However, it must be noted that the author now discourage the use of the attack method in favor of PGD for $\norm_{\infty}$~\footnote{Nicholas Carlini on \ac{CW} for $\norm_{\infty}$: \url{https://github.com/tensorflow/cleverhans/issues/978\#issuecomment-464594668}}.
For \ac{CW}, we had to limit the attack to 50 iterations as a measure to combat extreme runtime, that were infeasible to run on our available resources.
Thus the applied attack might not be able capture the full potential of the attack method.
Results of these experiments can be seen in Table~\ref{table:robustfgsm} and Table~\ref{table:robustcw}.
It can be seen that, despite having used PGD for the adversarial training, the improved robustness is also useful for perturbations of other attack methods.

\begin{table*}
  \setlength{\tabcolsep}{4pt}
  \sisetup{detect-all = true}
  \small
  \centering
  \begin{tabular}{
    l
    @{\hskip 2\tabcolsep}
    S[table-format=1.2, tight-spacing=true, table-text-alignment=left]
    *{3}{
    @{\hskip 2\tabcolsep}
    S[table-format=1.1, table-column-width=5em, table-align-uncertainty = false]
    S[table-format=1.1, table-column-width=5em, table-align-uncertainty = false]
    }}
    \toprule
     \parbox[t]{2mm}{\multirow{2}{*}{\rotatebox[origin=c]{90}{$\leftarrow$\small Loss}}} & \textbf{\ac{FGSM}} & \multicolumn{2}{c}{\textbf{CUB200-2011}} & \multicolumn{2}{@{}c@{\hskip 4\tabcolsep}}{\textbf{CARS196}} & \multicolumn{2}{@{}c@{}}{\textbf{SOP}} \\
    \cmidrule(lr{\dimexpr 4\tabcolsep-0.5em}){3-4} \cmidrule(l{-0.5em}r{\dimexpr 4\tabcolsep-0.5em}){5-6} \cmidrule(l{-0.5em}r{0.5em}){7-8}
   & & {R@1} & {mAP@R} & {R@1} & {mAP@R} & {R@1} & {mAP@R}\\
    \midrule
    \parbox[t]{2mm}{\multirow{2}{*}{C}} & \text{Natural} &           19.7 &                         7.2 &           14.6 &                         3.8 &           18.4 &                        10.8 \\

    & \textbf{Robust} & \bfseries 24.6 & \bfseries 9.9 & \bfseries 44.6 & \bfseries 12.4 & \bfseries 50.3 & \bfseries 29.2 \\
    \midrule
    \parbox[t]{2mm}{\multirow{2}{*}{T}} & \text{Natural} &           18.9 &                         7.7 &           15.5 &                         4.1 &           14.5 &                         8.5 \\
        & \textbf{Robust} & \bfseries 27.4 & \bfseries 11.0 & \bfseries 44.1 & \bfseries 13.0 & \bfseries 43.2 & \bfseries 24.2 \\
    \bottomrule
  \end{tabular}
  \caption{\label{table:robustfgsm}
    Performance of \ac{DML} models trained using the proposed adversarial training objective (using PGD) compared to naturally-trained \ac{DML} for adversarial perturbations within $\norm_{\infty}(\epsilon = 0.01)$ discovered using FGSM.
    Losses are denoted by C (contrastive) and T (triplet).
    The robustly trained model attain both higher inference accuracy (R@1) and improved ability to rank similar entities (mAP@R) than the naturally-trained baseline model.
    Thereby, the proposed robust training objective improves the robustness towards adversarial perturbations.
  }
\end{table*}

\begin{table*}
  \setlength{\tabcolsep}{4pt}
  \sisetup{detect-all = true}
  \small
  \centering
  \begin{tabular}{
    l
    @{\hskip 2\tabcolsep}
    S[table-format=1.2, tight-spacing=true, table-text-alignment=left]
    *{3}{
    @{\hskip 2\tabcolsep}
    S[table-format=1.1, table-column-width=5em]
    S[table-format=1.1, table-column-width=5em]
    }}
    \toprule
     \parbox[t]{2mm}{\multirow{2}{*}{\rotatebox[origin=c]{90}{$\leftarrow$\small Loss}}} & \textbf{\ac{CW}} & \multicolumn{2}{c}{\textbf{CUB200-2011}} & \multicolumn{2}{@{}c@{\hskip 4\tabcolsep}}{\textbf{CARS196}} & \multicolumn{2}{@{}c@{}}{\textbf{SOP}} \\
    \cmidrule(lr{\dimexpr 4\tabcolsep-0.5em}){3-4} \cmidrule(l{-0.5em}r{\dimexpr 4\tabcolsep-0.5em}){5-6} \cmidrule(l{-0.5em}r{0.5em}){7-8}
   & & {R@1} & {mAP@R} & {R@1} & {mAP@R} & {R@1} & {mAP@R}\\
    \midrule
    \parbox[t]{2mm}{\multirow{2}{*}{C}} & \text{Natural} &           15.1 &                         6.0 &            5.6 &                         2.3 &           23.1 &                        13.9 \\

    & \textbf{Robust} & \bfseries 37.4 & \bfseries 14.7 & \bfseries 58.6 & \bfseries 15.3 &  \bfseries 57.2 & \bfseries 32.6 \\
    \midrule
    \parbox[t]{2mm}{\multirow{2}{*}{T}} & \text{Natural} &           22.9 &                        10.0 &           13.4 &                         3.6 &           10.0 &                         6.1 \\
        & \textbf{Robust} & \bfseries 39.9 & \bfseries 16.2 & \bfseries 58.9 & \bfseries 16.0 & \bfseries 55.1 & \bfseries 32.2 \\
    \bottomrule
  \end{tabular}
  \caption{\label{table:robustcw}
    Performance of \ac{DML} models trained using the proposed adversarial training objective (using PGD) compared to naturally-trained \ac{DML} for adversarial perturbations within $\norm_{\infty}(\epsilon = 0.01)$ discovered using \ac{CW}.
    Losses are denoted by C (contrastive) and T (triplet).
    The robustly trained model attain both higher inference accuracy (R@1) and improved ability to rank similar entities (mAP@R) than the naturally-trained baseline model.
    Thereby, the proposed robust training objective improves the robustness towards adversarial perturbations.
  }
\end{table*}
