# Supplementary material for: Exploring Adversarial Robustness of Deep Metric Learning
Source: arXiv:2102.07265 source file (2021-02-14)
Supplement: Supplementary file 3 [file train_pert_target.tex]

\section{Experiment: Perturbation Target}\label{app:methods}
The proposed adversarial training techniques for \ac{DML} apply perturbations to positive data points.
This choice was made to establish alignment with the adversarial behavior covered in Section~\ref{sec:attackalg}.
However, the ``adversarial loss'' $\rho(\cdot,\cdot,\cdot)$ can capture violations across various data point types (anchor, positive, negative).
To assess the impact of using alternative perturbation targets (negative, anchor) for adversarial training, we performed an experiment with $P(\attackparam = 1) = 0.5$ (unless otherwise stated) across these alternative perturbation targets.
Losses and attack rates used during adversarial training, for the other perturbation targets, are specified below.

Negative perturbations for contrastive loss:
\[
  \lossfunc(\param, (\datapoint_{1} , y_{1} ), (\datapoint_{2} + \attackparam \rho_{(2,1)} ,y_{2})) \; \text{, }
\]
\[
  P(\attackparam = 1 \mid y_{1} = y_{2}) = 0 \; \text{, and } \; P(\attackparam = 1 \mid y_{1} \neq y_{2}) = 0.5 \; .
\]

Anchor perturbations for contrastive loss:
\[
  \lossfunc(\param, (\datapoint_{1} + \attackparam \rho_{(1,2)}, y_{1}), (\datapoint_{2}  ,y_{2})) \; \text{, }
\]
\[
  P(\attackparam = 1 \mid y_{1} = y_{2}) = P(\attackparam = 1 \mid y_{1} \neq y_{2}) = 0.5 \; .
\]

Negative perturbations for triplet loss:
\[
  \lossfunc(\param, (\datapoint_{1}, y_{1}), (\datapoint_{2}, y_{2}),(\datapoint_{3}  + \attackparam \rho_{(3,1)} ,y_{3}))
\]

Anchor perturbations for triplet loss:
\[
  \lossfunc(\param, (\datapoint_{1} + \attackparam \rho_{(1,2,3)}, y_{1}), (\datapoint_{2}, y_{2}),(\datapoint_{3}, y_{3}))
\]

Training processes for contrastive- and triplet loss can be seen in Figure~\ref{fig:conmethods} and Figure~\ref{fig:tripmethods}, respectively.
Across each combination of loss and dataset, the proposed adversarial training (positive perturbation) yields the most robustness for five out six experiments, with the exception of CUB200-2011 for contrastive loss.
Additionally, it reaches several orders of magnitudes higher performance on the CARS196 and SOP datasets.
We speculate that this inability for the alternative perturbation targets to reach similar performance can be linked to alterations on distance between anchors and negatives during training.
Having large distance between anchor data points and negative data points are known to cause instabilities during training, causing models to reach a local minima~\citep{wu17}.

\begin{figure}[ht]
  \includegraphics[width=\textwidth]{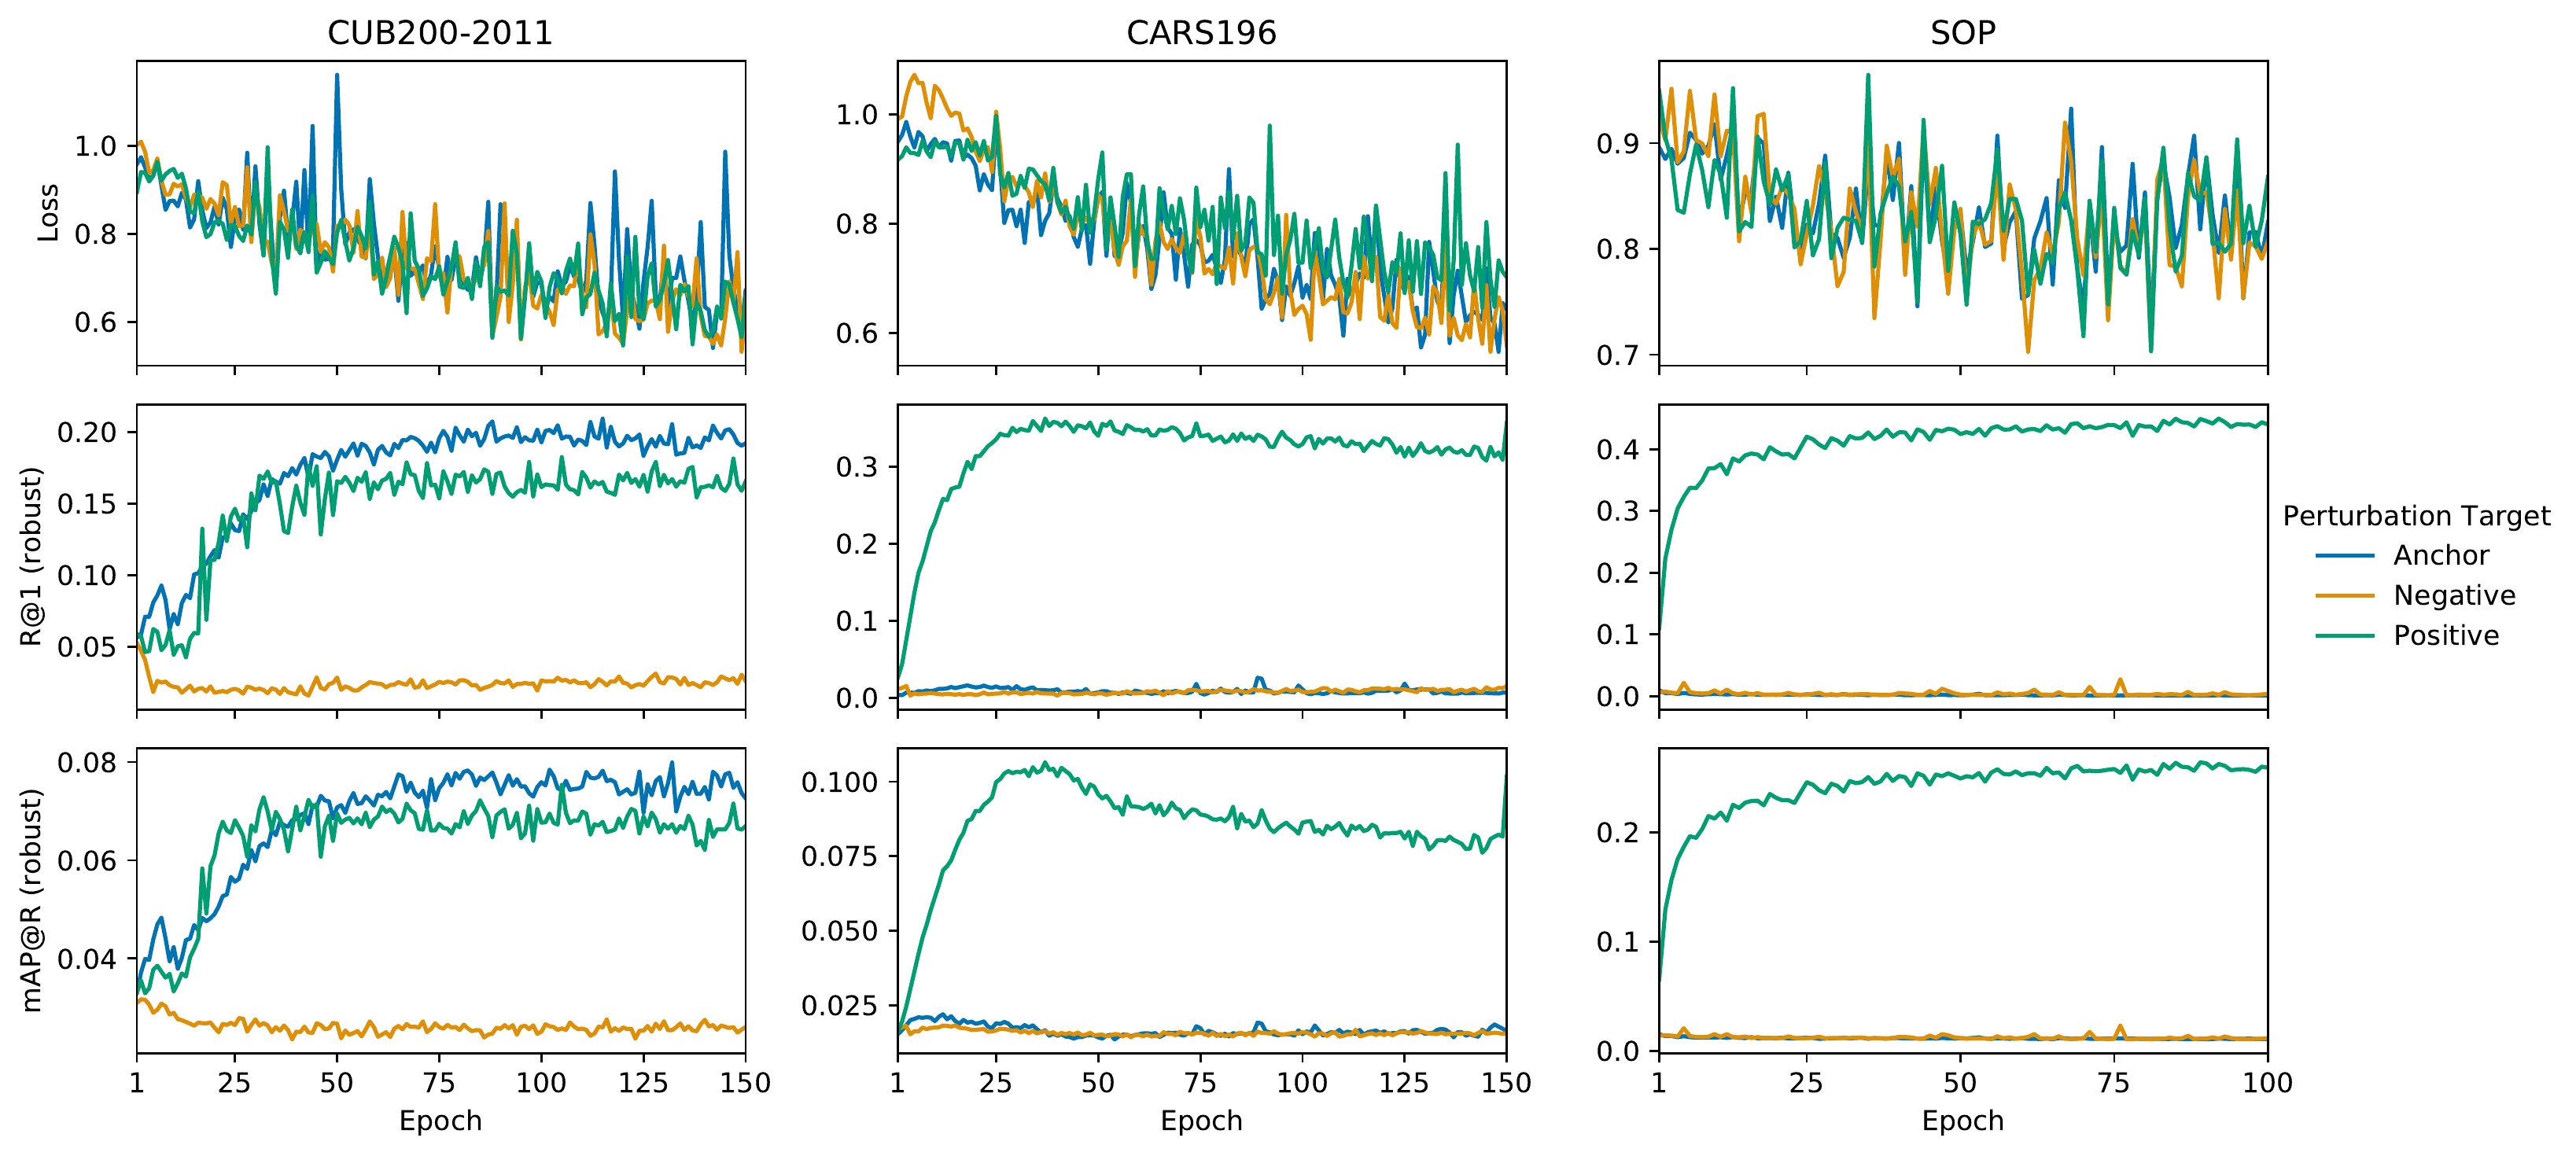}
  \caption{
    \label{fig:conmethods}
    Metrics (Loss, R@1, and mAP@R) for contrastive loss training procedure across perturbation targets.
    % The proposed method (positive) exceeds
    % Losses across perturbation targets, other than positive, does not greatly decrease as training progress, suggesting that the training has reached a local minima.
  }
\end{figure}

\begin{figure}[ht]
  \includegraphics[width=\textwidth]{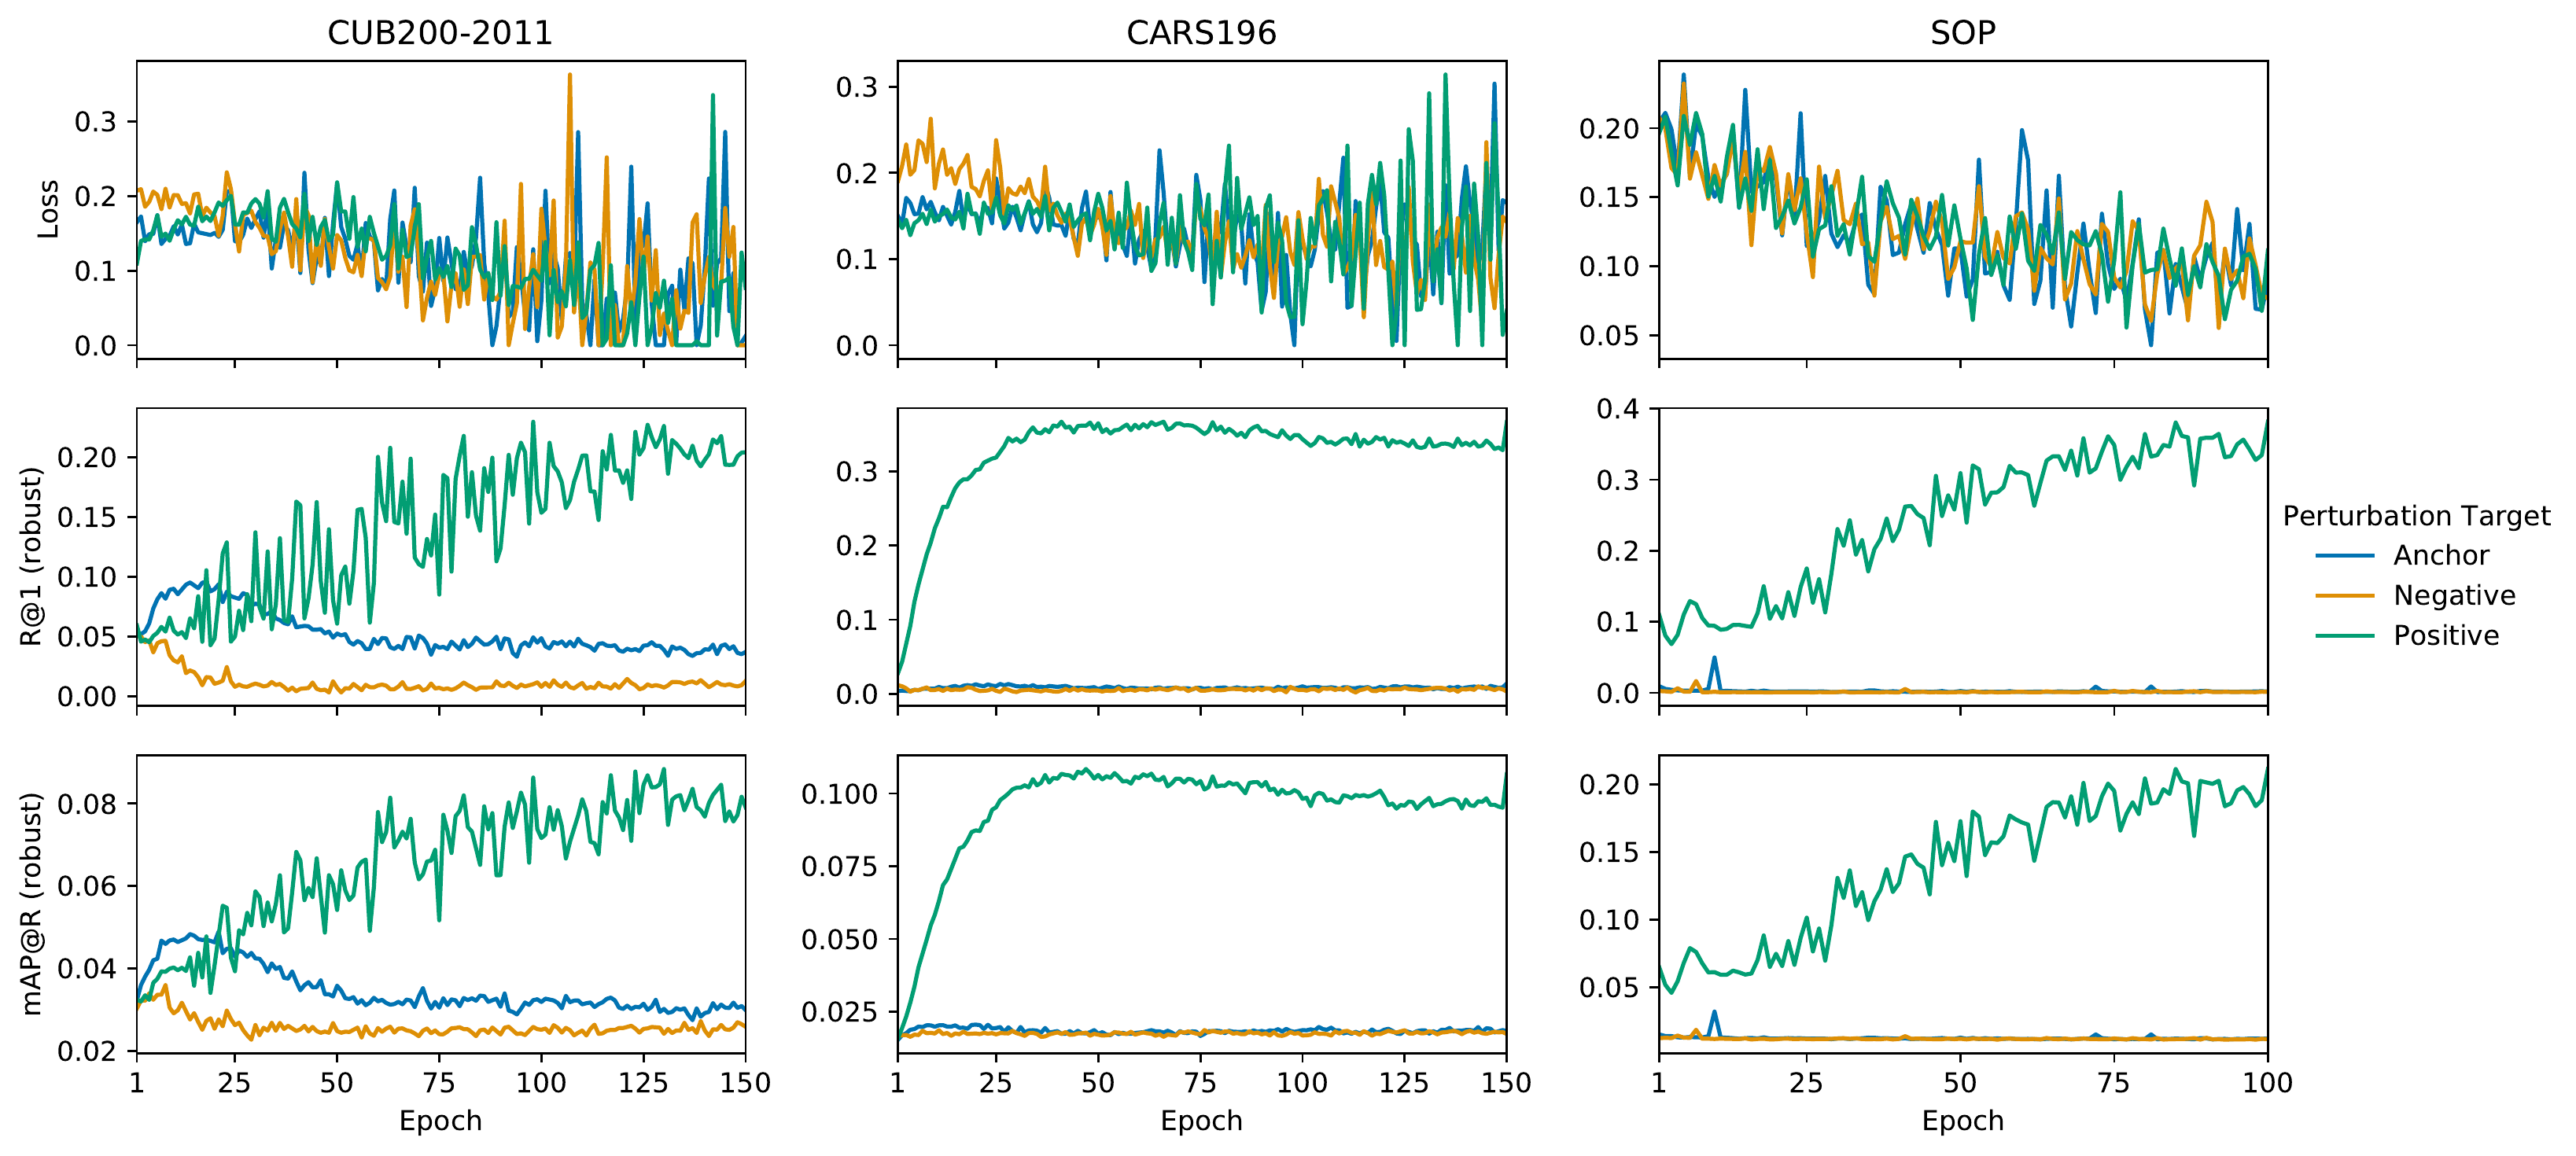}
  \caption{
    \label{fig:tripmethods}
    Metrics (Loss, R@1, and mAP@R) for triplet loss training procedure across perturbation targets.
  }
\end{figure}
