# Supplementary material for: Exploring Adversarial Robustness of Deep Metric Learning
Source: arXiv:2102.07265 source file (2021-02-14)
Supplement: Supplementary file 4 [file train_rates.tex]

\section{Experiment Details: Attack Rates}\label{app:rates}
This section expands upon the training process of the proposed robust formulation, particularly the impact of attack rate $P(\attackparam = 1)$, and the following performance of the \ac{DML} models.
In Table~\ref{table:robustrates}, the performance of models against adversarial perturbations across various attack rates can be seen.
These results demonstrate that robustness of the models being trained increases across all of the covered attack rates $P(\attackparam = 1) \in \{0.1, 0.25, 0.5, 0.75, 1.0\}$.
Additionally, there seems to be an association between higher attack rates yielding higher robustness.
However, this relationship is not monotonic, and across data sets and losses optimal choices for attack rate vary.
In Table~\ref{table:robustratesbenign}, the performance for the robust (and a naturally-trained) models against benign (unperturbed) input can be seen.
Generally, it can be seen that the robust formulation has minor impact on performance on benign input, as each model's evaluation metrics are close to performance of the naturally-trained baseline.
Interestingly, for contrastive loss on CUB200-2011 and CARS196 ($P(\attackparam = 1) = 0.25$ and $P(\attackparam = 1) = 0.1$), the robust training objective have enable the benign performance to exceed the naturally-trained baseline.
This could suggest that a low frequency of adversarial perturbations could potentially improve the training process of non-robust \ac{DML}.
We deem more details on this to out of scope for our work, but see it as an promising direction for future research to explore more thoroughly.

\begin{table}
  \setlength{\tabcolsep}{4pt}
  \sisetup{detect-all = true}
  \small
  \centering
  \begin{tabular}{
    l
    @{\hskip 2\tabcolsep}
    S[table-format=1.2, tight-spacing=true, table-text-alignment=left]
    *{3}{
    @{\hskip 4\tabcolsep}
    S[table-format=2.1, table-column-width=4em]
    S[table-format=2.1, table-column-width=4em]
    }}
    \toprule
    & & \multicolumn{2}{c}{\textbf{CUB200-2011}} & \multicolumn{2}{@{}c@{\hskip 4\tabcolsep}}{\textbf{CARS196}} & \multicolumn{2}{@{}c@{}}{\textbf{SOP}} \\
    \cmidrule(lr{\dimexpr 4\tabcolsep-0.5em}){3-4} \cmidrule(l{-0.5em}r{\dimexpr 4\tabcolsep-0.5em}){5-6} \cmidrule(l{-0.5em}r{0.5em}){7-8}
   \multicolumn{2}{l}{$P(\attackparam = 1)\downarrow$} & {R@1} & {mAP@R} & {R@1} & {mAP@R} & {R@1} & {mAP@R}\\
    \midrule
    \parbox[t]{2mm}{\multirow{6}{*}{\rotatebox[origin=c]{90}{Contrastive}}} & \textit{Naturally-trained} &     2.1 \pm 0.1 &                 2.6 \pm 0.0 &    0.4 \pm 0.0 &                 1.5 \pm 0.0 &    1.3 \pm 0.0 &                 1.7 \pm 0.0 \\
    \cmidrule(l{-0.5em}r{0.0em}){2-8}
& 0.1 &             8.0 &                         4.0 &             8.5 &                         2.7 &            21.3 &                        12.2 \\
        & 0.25 &            17.9 &                         6.8 &            27.1 &                         7.2 &            39.8 &                        23.7 \\
        & 0.5 &  \bfseries 18.4 &               \bfseries 7.5 &            35.7 &                        10.2 &            44.9 &                        26.2 \\
        & 0.75 &  \bfseries 18.4 &                         7.3 &            39.5 &                        11.4 &  \bfseries 48.7 &              \bfseries 28.3 \\
        & 1.0 &            15.4 &                         6.5 &  \bfseries 41.4 &              \bfseries 11.5 &            44.0 &                        24.9 \\
    \midrule
    \parbox[t]{2mm}{\multirow{6}{*}{\rotatebox[origin=c]{90}{Triplet}}} & \textit{Naturally-trained} &     2.5 \pm 0.1 &                 3.0 \pm 0.0 &    0.3 \pm 0.0 &                 1.6 \pm 0.0 &    0.5 \pm 0.0 &                 1.4 \pm 0.0 \\
    \cmidrule(l{-0.5em}r{0.0em}){2-8}
& 0.1 &            22.3 &               \bfseries 8.8 &            29.7 &                         8.0 &            26.8 &                        15.2 \\
        & 0.25 &            22.1 &               \bfseries 8.8 &            32.7 &                         9.2 &            32.2 &                        18.4 \\
        & 0.5 &  \bfseries 23.1 &                         8.6 &            36.7 &                        10.7 &  \bfseries 38.1 &              \bfseries 21.1 \\
        & 0.75 &            20.4 &                         7.7 &            39.7 &                        11.6 &  \bfseries 38.1 &                        20.9 \\
        & 1.0 &             8.7 &                         3.7 &  \bfseries 40.6 &              \bfseries 11.9 &            28.8 &                        15.4 \\
    \bottomrule
  \end{tabular}
  \caption{\label{table:robustrates}
    Performance of robust \ac{DML} models on adversarial input for various specified (training) attack rates $P(\attackparam = 1)$ .
    These models were trained using the proposed adversarial training algorithm (covered in Section~\ref{sec:advtrain}) with PGD for $\norm_{\infty}(\epsilon = 0.01)$.
    Evaluations on conducted on adversarial input generated using Algorithm~\ref{alg:attack}.
    Naturally-trained marks the performance of \ac{DML} models using traditional non-robust training objectives.
    \textbf{Bold} marks best performance for dataset, metric, loss combinations.
    Robust models reach higher inference accuracy (R@1) and better ability to rank similar entities (mAP@R) on adversarial input than naturally-trained \ac{DML} models.
    Higher attack rates are often associated with higher robustness.
  }
\end{table}

\begin{table}
  \setlength{\tabcolsep}{4pt}
  \sisetup{detect-all = true}
  \small
  \centering
  \begin{tabular}{
    l
    @{\hskip 2\tabcolsep}
    S[table-format=1.2, tight-spacing=true, table-text-alignment=left]
    *{3}{
    @{\hskip 4\tabcolsep}
    S[table-format=2.1, table-column-width=4em]
    S[table-format=2.1, table-column-width=4em]
    }}
    \toprule
    & & \multicolumn{2}{c}{\textbf{CUB200-2011}} & \multicolumn{2}{@{}c@{\hskip 4\tabcolsep}}{\textbf{CARS196}} & \multicolumn{2}{@{}c@{}}{\textbf{SOP}} \\
    \cmidrule(lr{\dimexpr 4\tabcolsep-0.5em}){3-4} \cmidrule(l{-0.5em}r{\dimexpr 4\tabcolsep-0.5em}){5-6} \cmidrule(l{-0.5em}r{0.5em}){7-8}
   \multicolumn{2}{l}{$P(\attackparam = 1)\downarrow$} & {R@1} & {mAP@R} & {R@1} & {mAP@R} & {R@1} & {mAP@R}\\
    \midrule
    \parbox[t]{2mm}{\multirow{6}{*}{\rotatebox[origin=c]{90}{Contrastive}}} & \textit{Naturally-trained} &   \itshape 59.1 \pm 0.0 &                \itshape 21.0 \pm 0.0 &  \itshape 74.0 \pm 0.0 & \bfseries \itshape 20.9 \pm 0.0 & \bfseries \itshape 71.8 \pm 0.0 & \bfseries \itshape 44.7 \pm 0.0 \\
    \cmidrule(l{-0.5em}r{0.0em}){2-8}
& 0.1 &            54.5 &                        17.2 &  \bfseries 74.4 &              \bfseries 20.9 &  69.7 &               42.2 \\
        & 0.25 &  \bfseries 60.1 &              \bfseries 21.9 &            74.0 &                        20.3 &            66.7 &                        39.2 \\
        & 0.5 &            52.1 &                        15.8 &            71.8 &                        18.3 &            65.1 &                        37.3 \\
        & 0.75 &            50.7 &                        14.8 &            70.1 &                        17.3 &            62.0 &                        34.4 \\
        & 1.0 &            48.3 &                        13.2 &            67.7 &                        15.9 &            59.7 &                        32.1 \\
    \midrule
    \parbox[t]{2mm}{\multirow{6}{*}{\rotatebox[origin=c]{90}{Triplet}}} & \textit{Naturally-trained} &  \bfseries \itshape 59.3 \pm 0.0 &     \bfseries  \itshape 21.7 \pm 0.0 &  \bfseries \itshape 74.0 \pm 0.0 & \bfseries \itshape 21.4 \pm 0.0 &  \bfseries \itshape 69.6 \pm 0.0 &  \bfseries \itshape42.1 \pm 0.0 \\
    \cmidrule(l{-0.5em}r{0.0em}){2-8}
& 0.1 &            51.7 &                        16.9 &  72.2 &               19.2 &  67.0 &               39.1 \\
        & 0.25 &            52.2 &                        16.8 &            70.9 &                        18.4 &            65.2 &                        37.2 \\
        & 0.5 &  53.8 &              17.4 &            71.7 &                        18.9 &            64.9 &                        36.6 \\
        & 0.75 &            53.0 &                        16.5 &            70.3 &                        18.1 &            63.5 &                        35.3 \\
        & 1.0 &            47.5 &                        13.0 &            70.2 &                        17.3 &            56.7 &                        29.0 \\
    \bottomrule
  \end{tabular}
  \caption{\label{table:robustratesbenign}
    Performance of robust \ac{DML} models on benign input for various specified (training) attack rates $P(\attackparam = 1)$ .
    These models were trained using the proposed adversarial training algorithm (covered in Section~\ref{sec:advtrain}) with PGD for $\norm_{\infty}(\epsilon = 0.01)$.
    Evaluations on benign data.
    Naturally-trained marks the performance of \ac{DML} models using traditional non-robust training objectives.
    \textbf{Bold} marks best performance for dataset, metric, loss combinations.
    Higher attack rates are often associated with lower performance on benign input.
    For contrastive loss
  }
\end{table}
