# Supplementary material for: Exploring Adversarial Robustness of Deep Metric Learning
Source: arXiv:2102.07265 source file (2021-02-14)
Supplement: Supplementary file 5 [file train_synthetic.tex]

\section{Experiment: Synthetic Data}~\label{app:synthetic}
As a measure to establish more clarity into the effects of induced by the robust training objective (covered in Section~\ref{sec:background}), we seek to construct an experiment with two high-dimensional and well-defined data distributions being mapped to low-dimensional embedding space.
We define the dimensionality of the high-dimensional input space as $k = 3 \times 224 \times 224$, in order to share the dimensionality of the other experiments using real-world datasets.
We construct the dataset with two classes, ``a'' and ``b'', for which each has an associated independent $k$-dimensional Gaussian distribution.
These distributions are $\mathcal{N}_{k}(\mu_{a}, \mathbf{\Sigma})$ and $\mathcal{N}_{k}(\mu_{b}, \mathbf{\Sigma})$, for class ``a'' and ``b'' respectively, where:
\begin{equation}
    \mu_{a} = \begin{pmatrix}0.25 & \cdots & 0.25\end{pmatrix} \in \mathbb{R}^{k}\text{,}
    \quad \mu_{b} = \begin{pmatrix}0.75 & \cdots & 0.75\end{pmatrix} \in \mathbb{R}^{k}\; \text{, and} \;
    \; \mathbf{\Sigma} = \sigma^{2} \cdot I_{k} \;.
\end{equation}

Here, $I_{k} \in \mathbb{R}^{k \times k}$ is the identity matrix of size $k$ and $\sigma = 0.025$.
Following this, we draw a dataset $D_{\mathcal{N}}$ with a fixed amount of data points for each class and train a deep metric model $\encfunc \colon \mathbb{R}^{k} \to \mathbb{R}^{2}$ parameterized by $\param$.
We choose to have the embedding space be two-dimensional as a measure to enable visualizations of the learned embedding space.
Using $D_{\mathcal{N}}$, we train two variants of $\encfunc$, one using the natural (non-robust) training objective and another using the proposed robust training objective (for $\ell_{\infty}(\epsilon = 0.01)$).
Each model use contrastive loss, is trained across 25 epochs on 508 train data points, while being evaluated on 516 test data points.
Following, we perform a test-time attack using Algorithm~\ref{alg:attack} with PGD ($\epsilon = 0.01$).
Differences of the learned embedding spaces, and the influence of the adversarial perturbations, can be seen in Figure~\ref{fig:synthetic}.

\begin{figure}[ht]
  \centering
  \includegraphics[width=.8\textwidth]{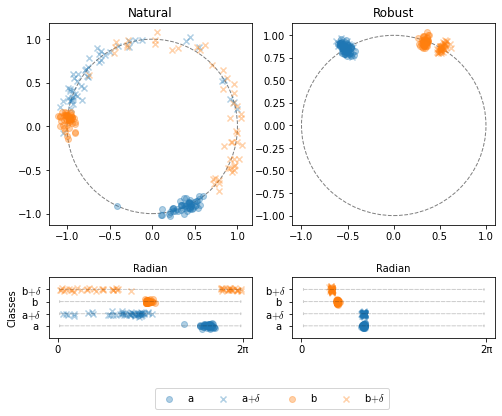}
  \label{fig:synthetic}
  \caption{
    Effects of adversarial perturbations in the embedding space (embedding shift, inference) for 16 randomly sampled data points.
    Circles mark embeddings of unperturbed data points, while crosses are adversarial perturbations for the respective data points.
    (first row) Grey lines connect the unperturbed data points to their perturbed counterpart, to highlight the shift in the embedding space.
    (second row) Green and red lines connect the embedding of the respective adversarial data point to its nearest (and unperturbed) neighbor.
    If the line is green, this neighbor is of the same class (correct) while red is the opposite (wrong).
    It can be seen that embeddings of the robustly-trained model shifts much less, when faced with adversarial perturbed input, and are thus more robust.
  }
\end{figure}

Generally, it can be seen that embeddings of the robust model remain more stable (in terms of position) in the embedding space, when compared to naturally-trained model.
Both models have $\text{R@1} = 100.0$ for benign (unperturbed) data, while the naturally-trained model have $\text{R@1} = 4.6$ for adversarial data points, while the robust model attains $\text{R@1} = 100.0$ for those data points.
